# Supplementary material for: WhiteLie: A Robust System for Spoofing User Data in Android Platforms
Source: arXiv:2512.01595 source file (2025-12-01)
Supplement: Supplementary file 1 [file A_Appendix.tex]

% \onecolumn 
% \refstepcounter{appendixa}
\section{Memory Used by Various Processes during Micro-Benchmarking}
\label{sec:appendixA}

\begin{figure}[htbp]
\centering
\begin{subfigure}{0.89\textwidth}
    \includegraphics[width=\textwidth]{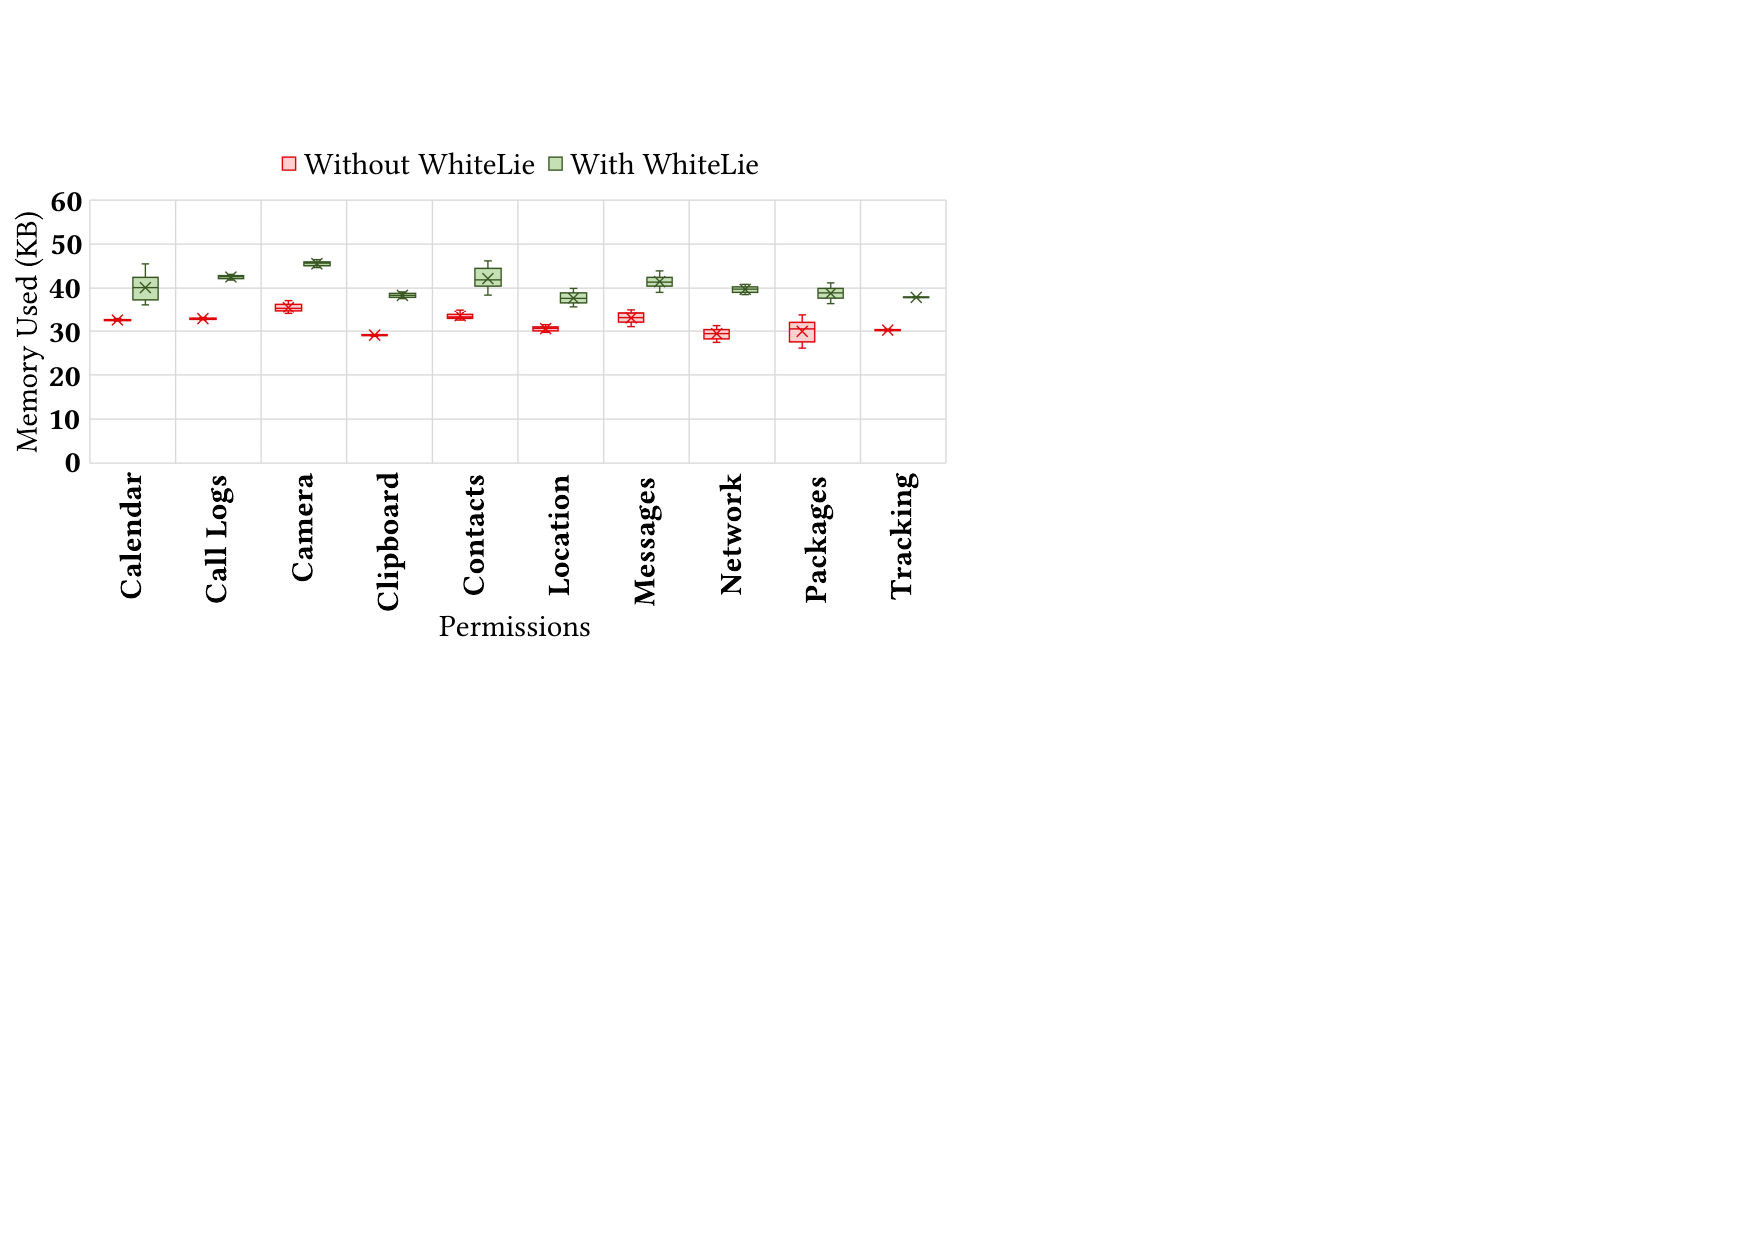}
    \caption{Target App}
    \label{fig:reslts_mem_target_app}
\end{subfigure}
\begin{subfigure}{0.89\textwidth}
    \includegraphics[width=\textwidth]{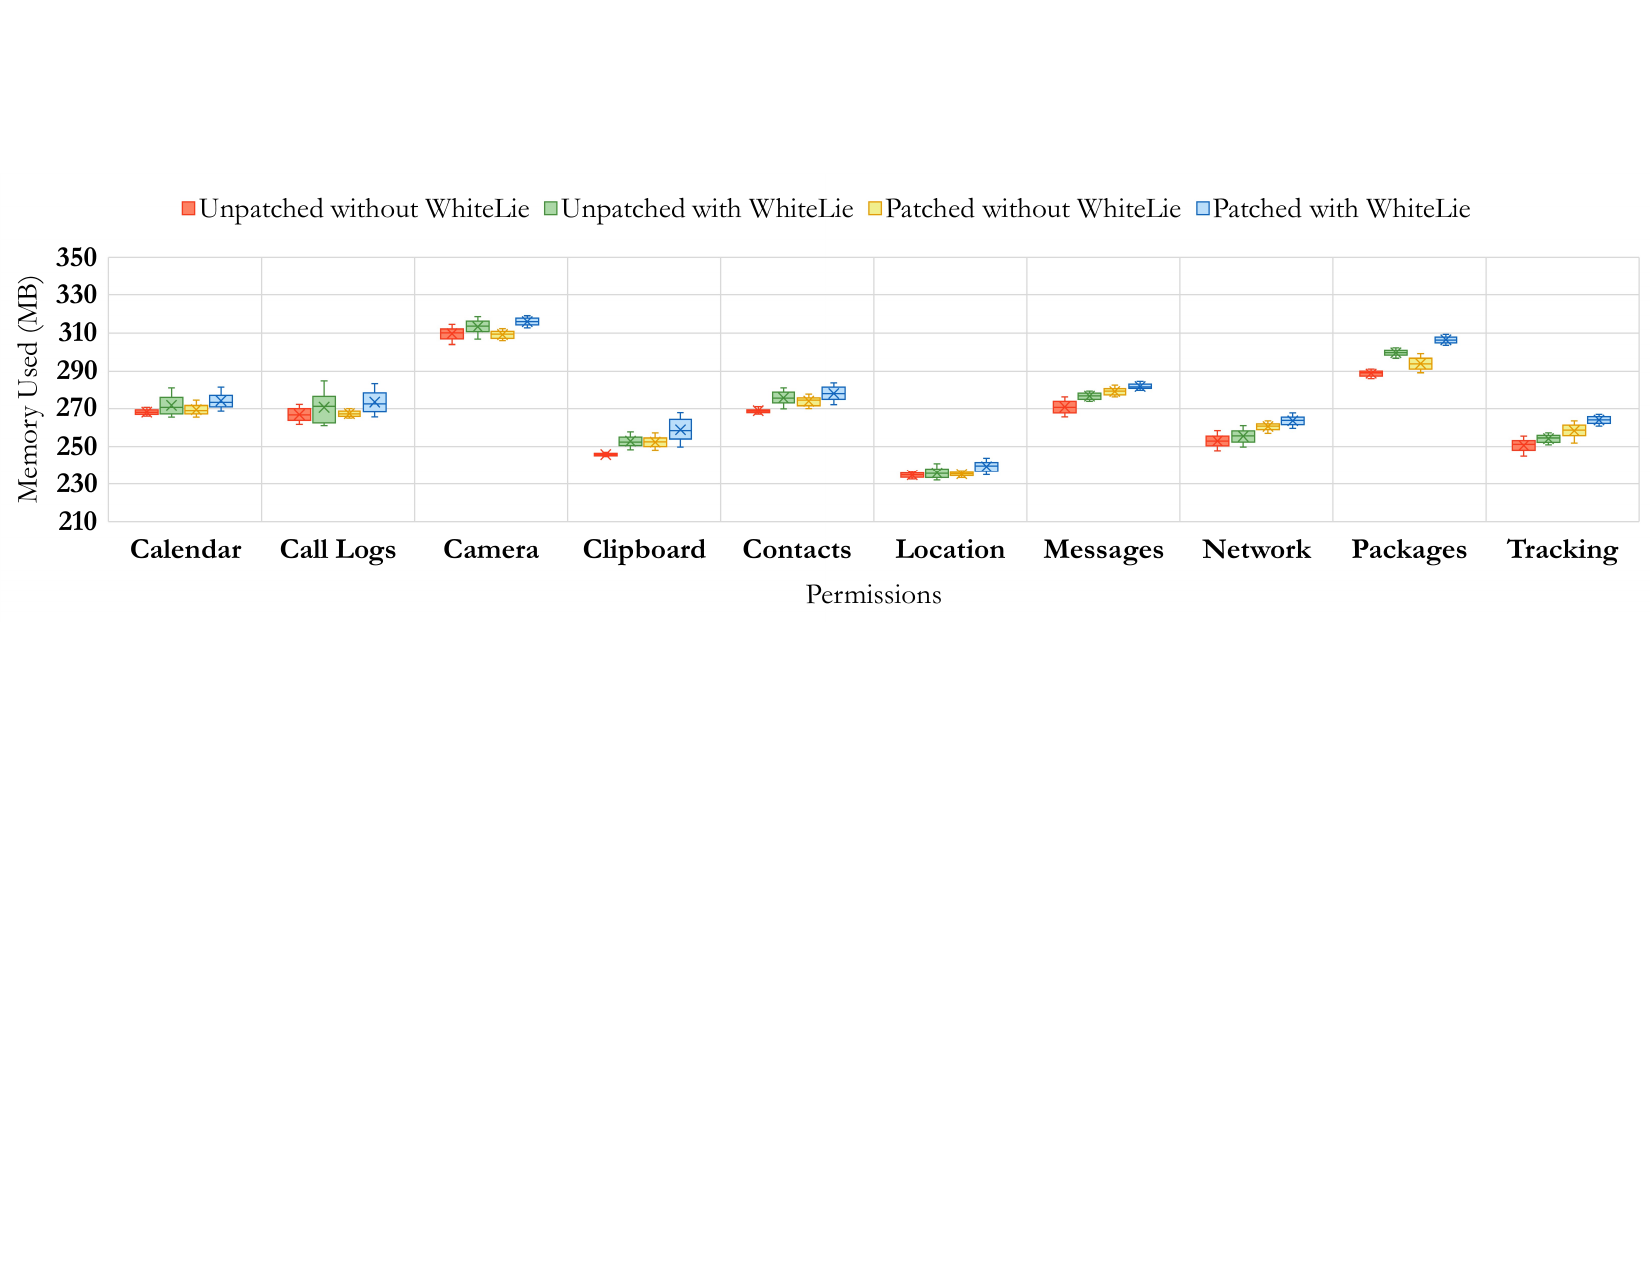}
    \caption{System}
    \label{fig:reslts_mem_sys}
\end{subfigure}

\begin{subfigure}{0.89\textwidth}
    \includegraphics[width=\textwidth]{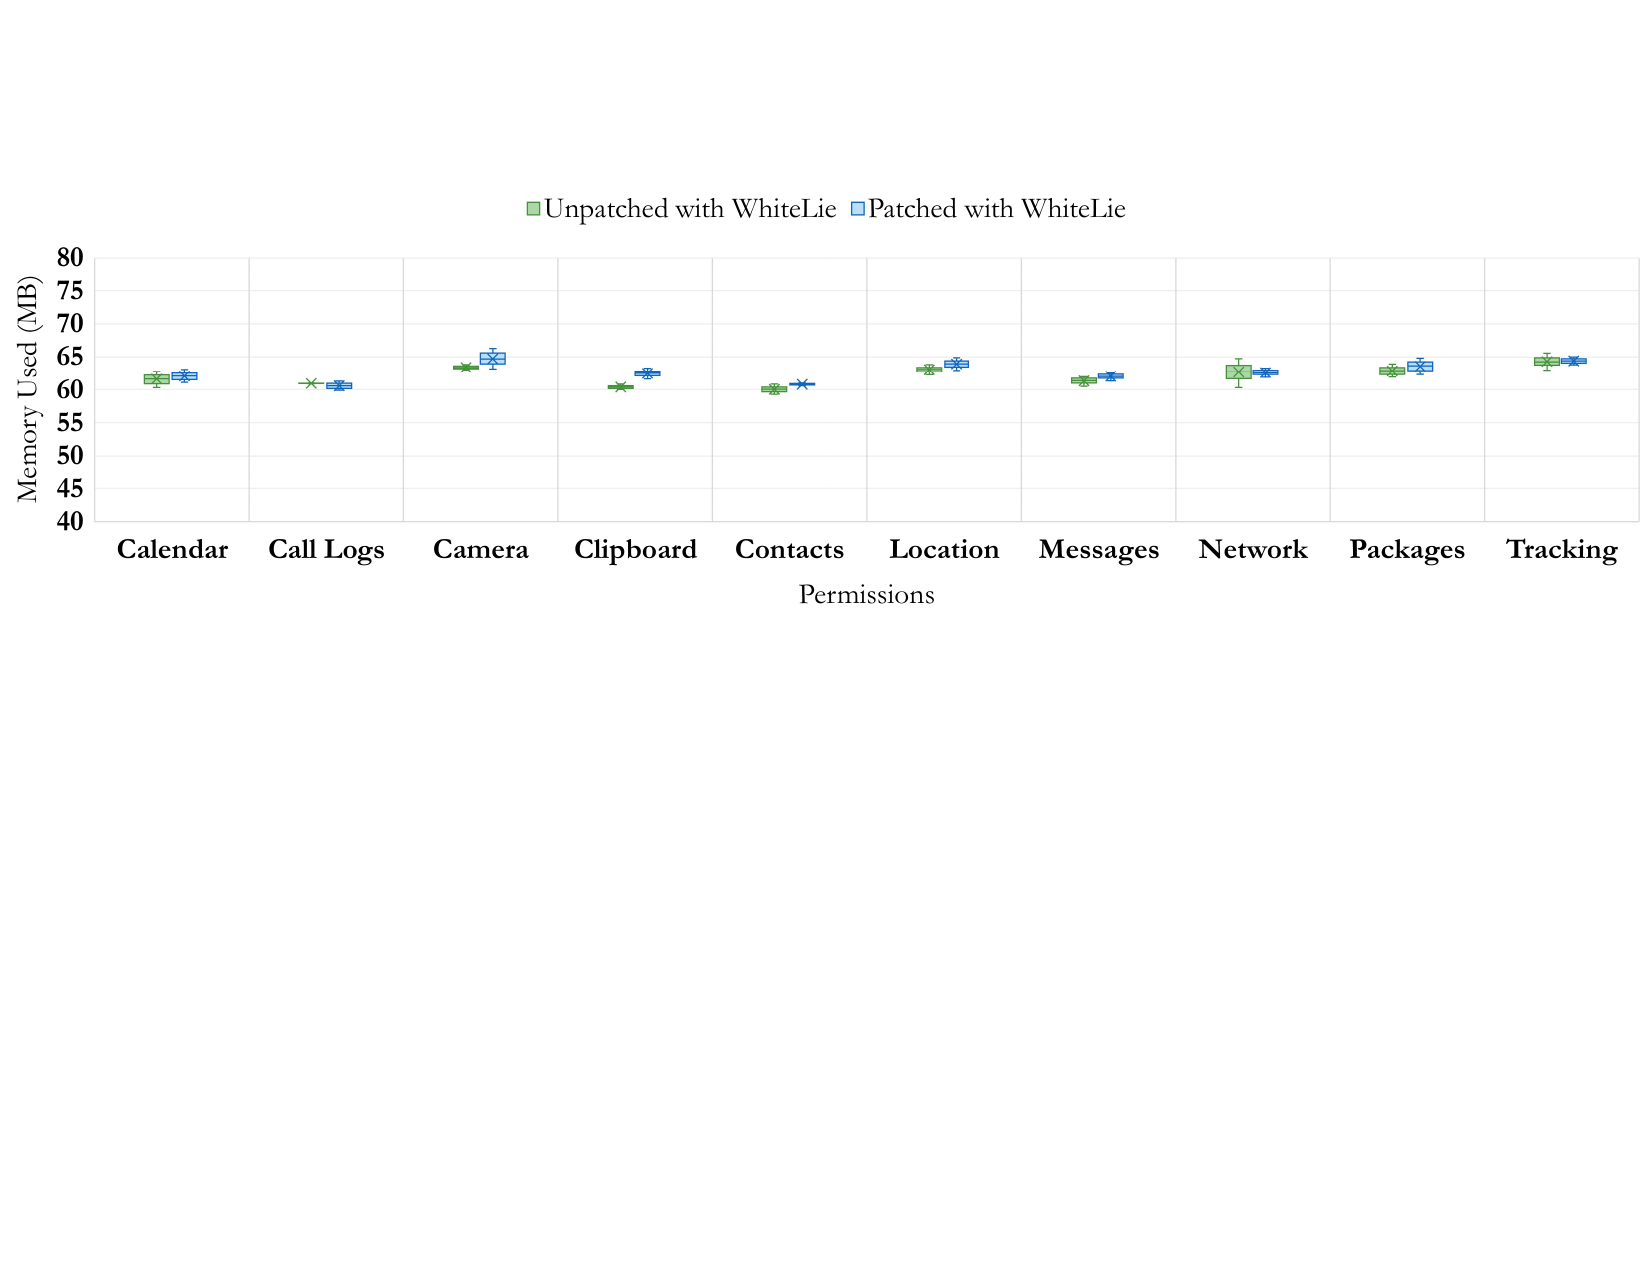}
    \caption{\framework{}}
    \label{fig:reslts_mem_frmwrk}
\end{subfigure}

\begin{subfigure}{0.89\textwidth}
    \includegraphics[width=\textwidth]{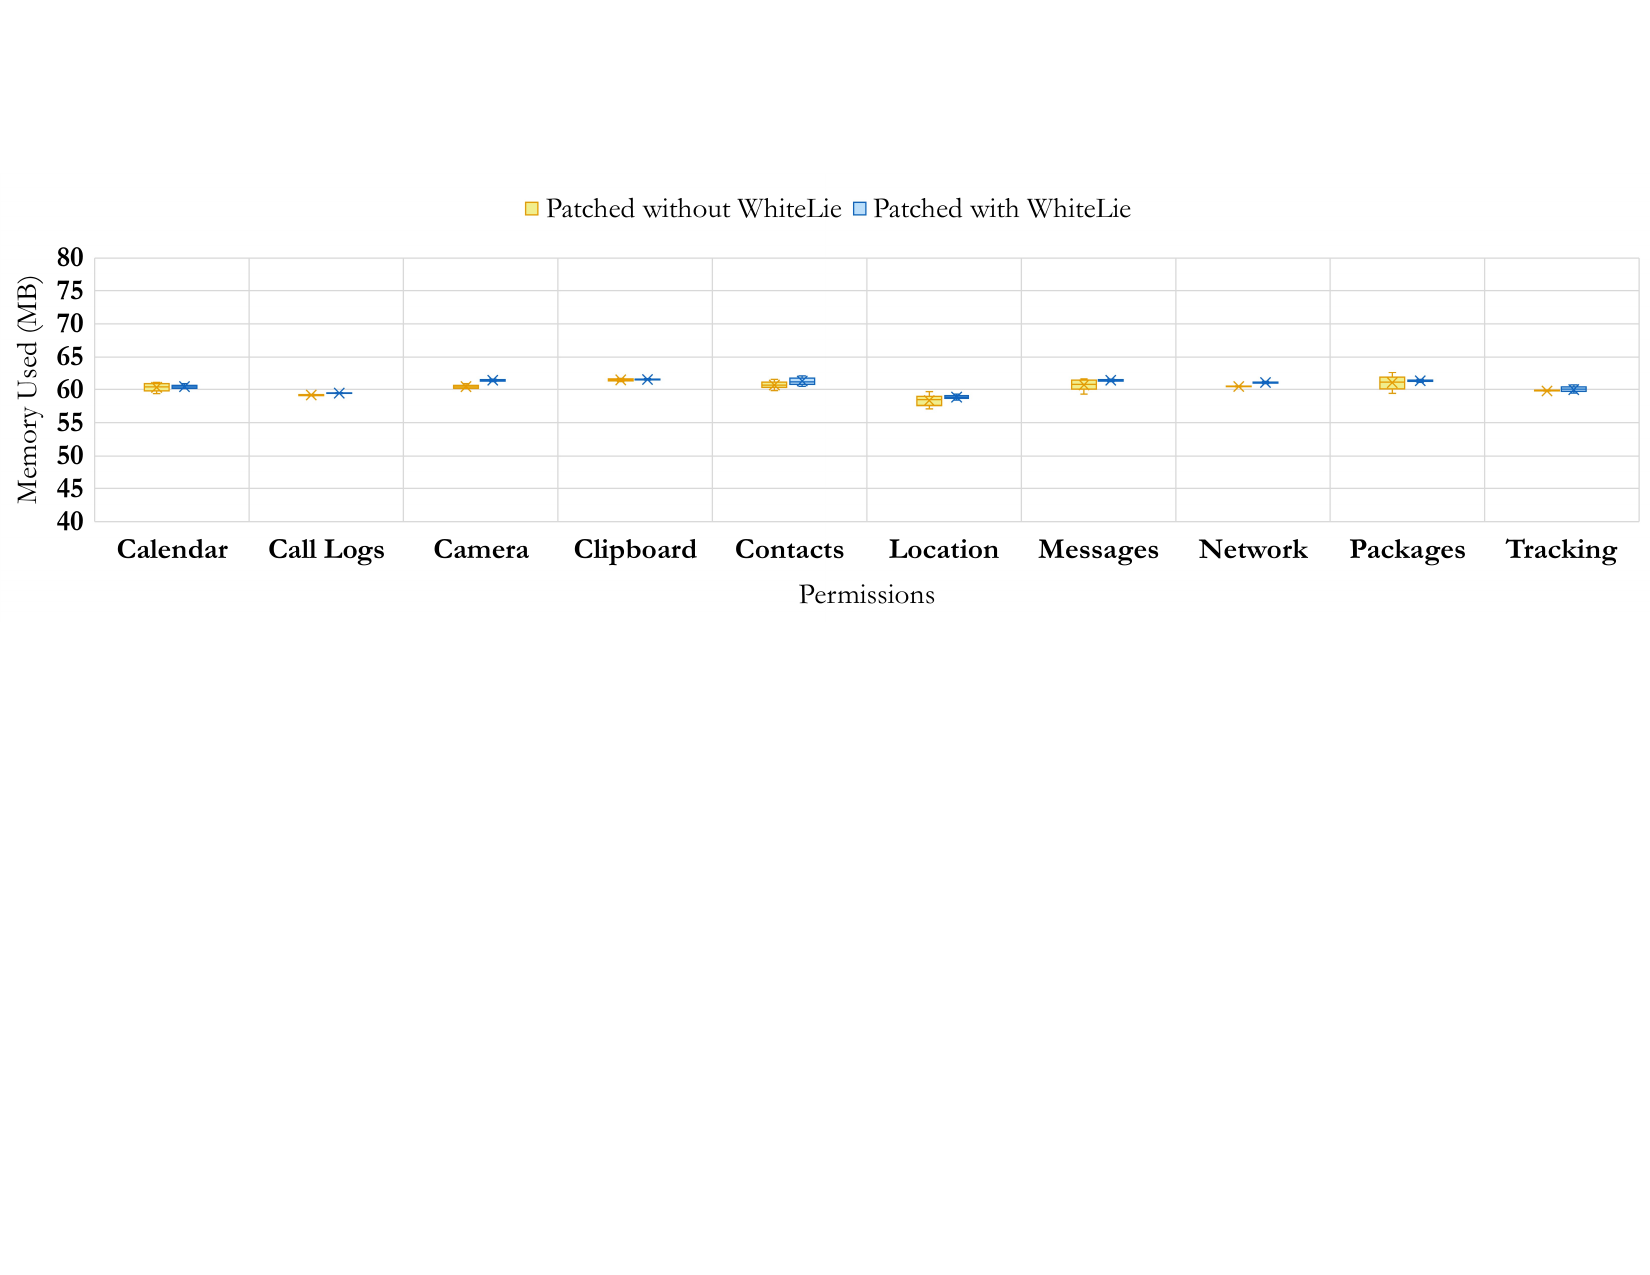}
    \caption{Patcher}
    \label{fig:reslts_mem_ptchr}
\end{subfigure}

\caption{Memory used by various processes involved in experimentation for various Permissions in different configurations}
\label{fig:results_memUsed}
\end{figure}
