# Supplementary material for: WhiteLie: A Robust System for Spoofing User Data in Android Platforms
Source: arXiv:2512.01595 source file (2025-12-01)
Supplement: Supplementary file 2 [file B_Appendix.tex]

\begin{figure*}[t]
    \includegraphics[width=\linewidth]{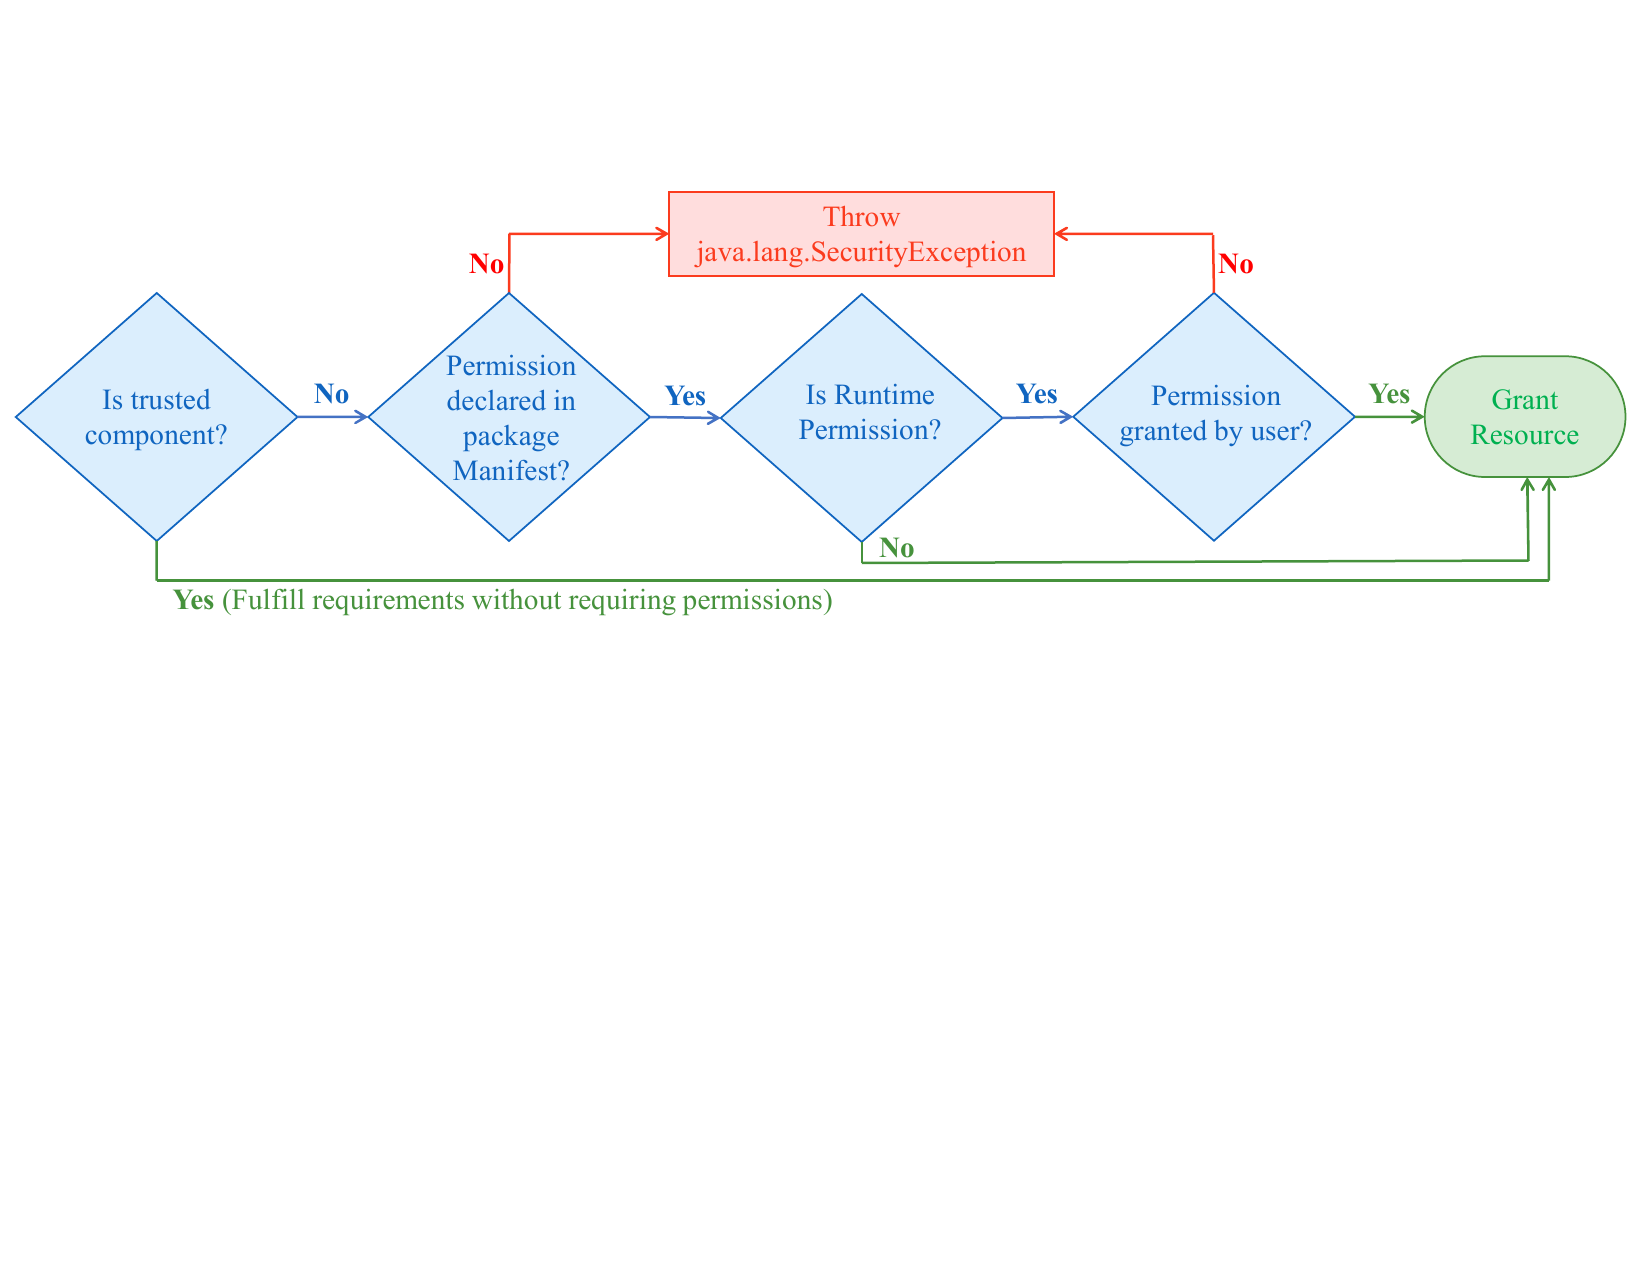}
    \caption{Android permission framework.}
    \label{fig:bg_andPermFrmwrkWrkng}
\end{figure*}

\begin{figure*}[htbp]
\includegraphics[width=\linewidth]{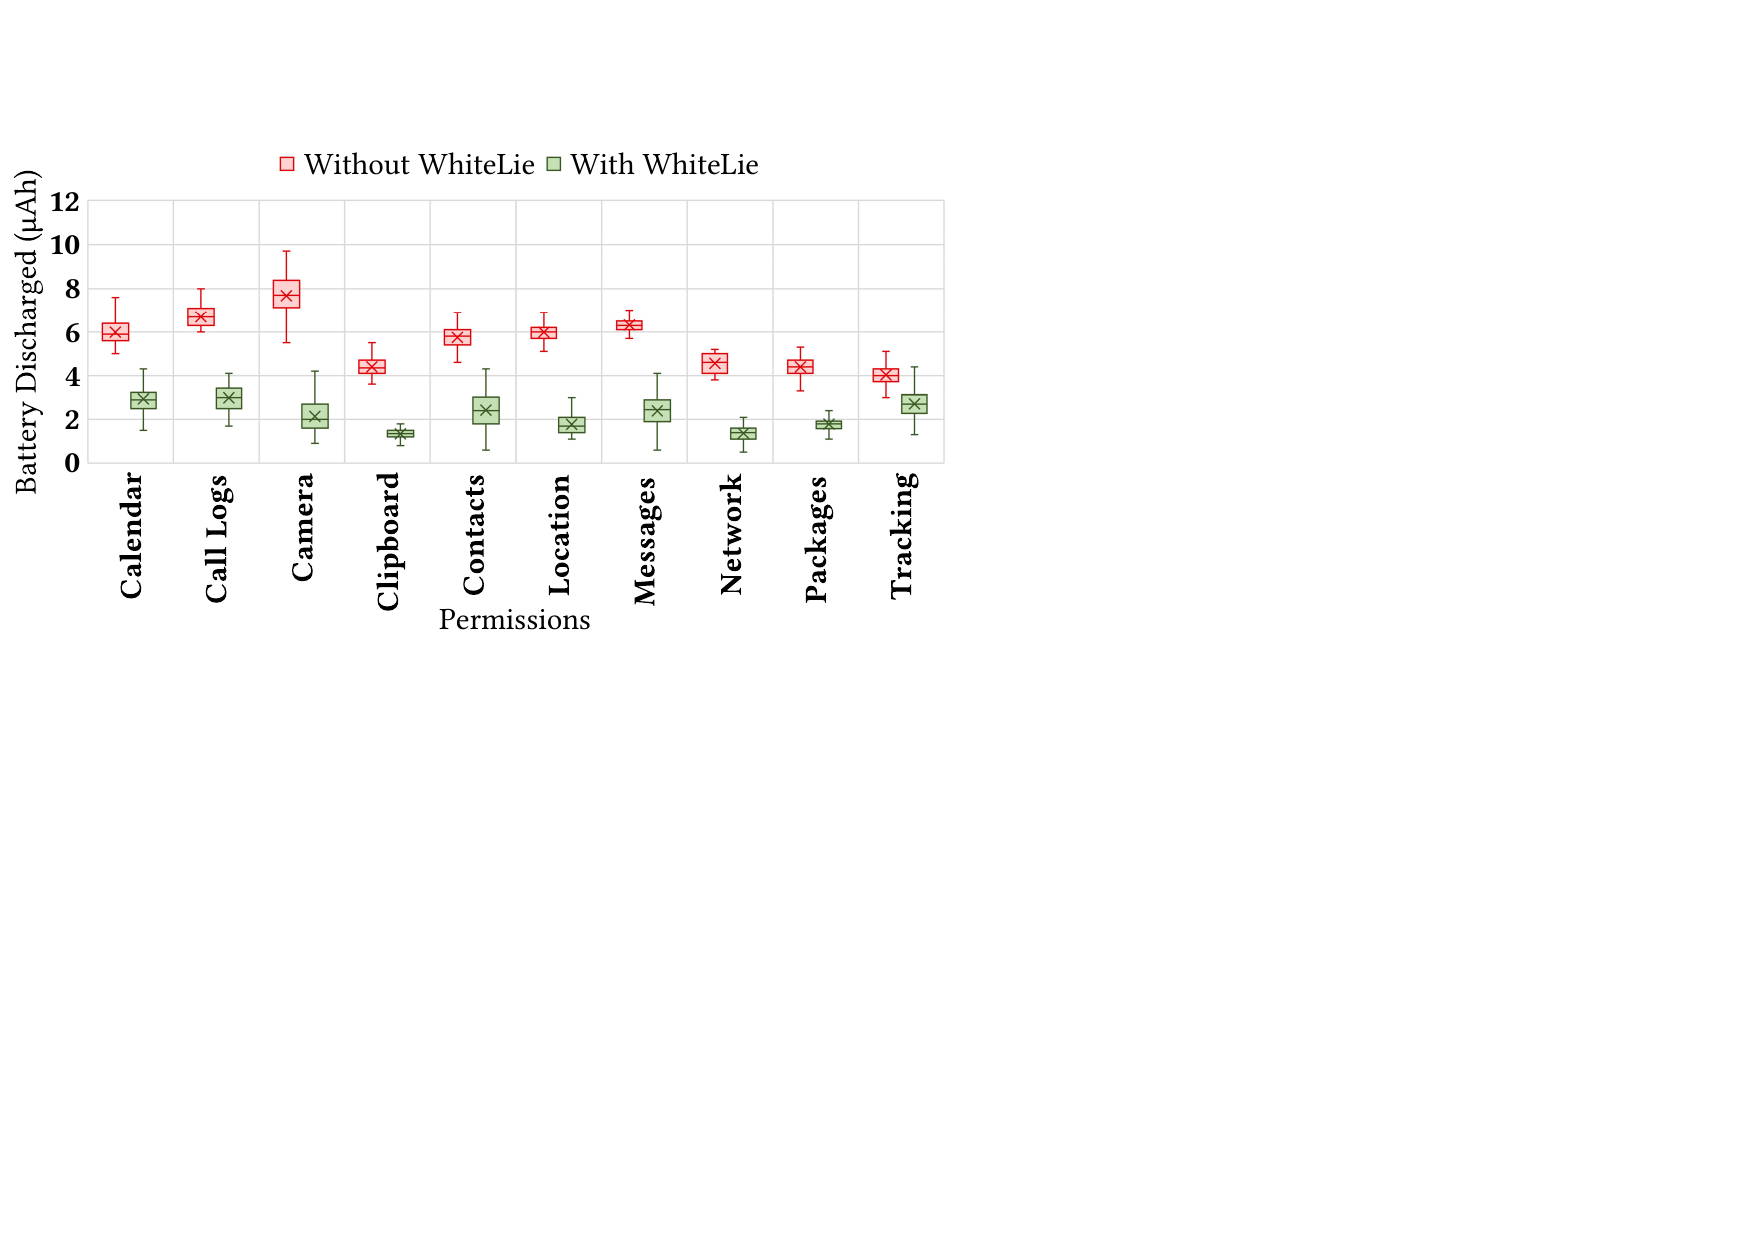}
\caption{Battery Discharged for various Permissions in different configurations with \framework{}'s \textit{Battery Saver}}
\label{fig:discus_btrySavr}
\end{figure*}
